# Supplementary material for: Quantized electrical, thermal, and spin transports of non-Hermitian clean and dirty two-dimensional topological insulators and superconductors
Source: arXiv:2408.00763 ancillary file (2024-12-04)
Supplement: Supplementary file 1 [file Supplementary_NHTransport.pdf]

# Supplemental Material:
# Quantized electrical, thermal, and spin transports of non-Hermitian clean and dirty two-dimensional topological insulators and superconductors

Sanjib Kumar Das[1] and Bitan Roy[1]

[1] *Department of Physics, Lehigh University, Bethlehem, Pennsylvania, 18015, USA*

(Dated: August 1, 2024)

This Supplemental Material contains (a) details of the transport calculations using scattering matrix theory in Kwant [Sec. S1], and (b) details of the numerical simulations of electrical, thermal, and spin transport quantities in disordered systems [Sec. S2 and Figs. S1- S3].

## S1. TRANSPORT CALCULATIONS FROM SCATTERING MATRIX THEORY

In this section, we present some additional details related to the transport calculations that use the scattering matrix theory in Kwant software package to compute the electrical, thermal, and spin transport properties of two-dimensional non-Hermitian (NH) topological insulators and superconductors. The rectangular scattering region (system) is attached to six leads. All the leads are semi-infinite and they supply fermions to the scattering region.

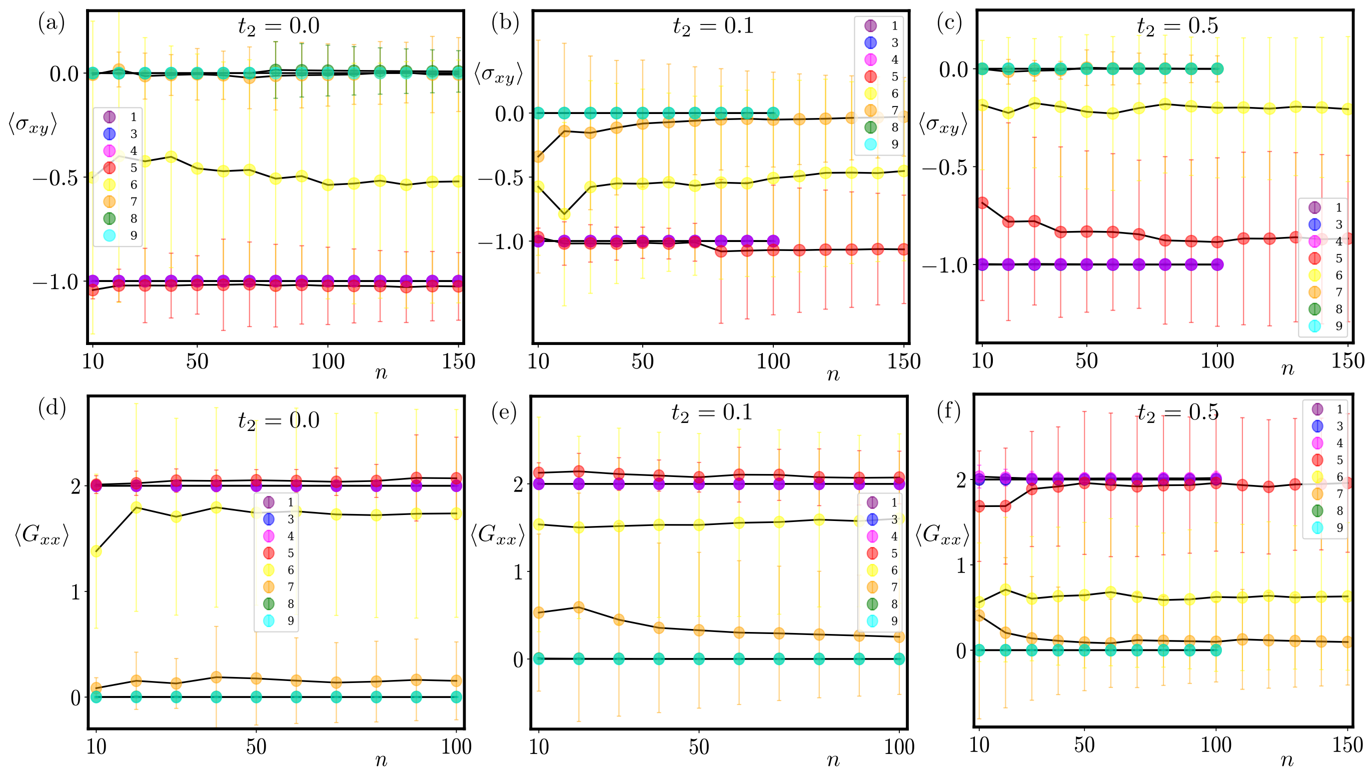


Figure S1. The variation of the disorder-averaged electrical Hall conductivity $\langle \sigma_{xy} \rangle$ in NH QAHI with the number of independent disorder realizations $n$ for (a) $t_2 = 0.0$, (b) $t_2 = 0.1$, and (c) $t_2 = 0.5$ for a few specific values of the disorder strength ($W$), quoted in the legend of each subfigure. The variation of the disorder-averaged electrical longitudinal conductivity $\langle G_{xx} \rangle$ in NH QSHI with the number of independent disorder realizations ($n$) for (d) $t_2 = 0.0$, (e) $t_2 = 0.1$, and (f) $t_2 = 0.5$ for a few specific values of the disorder strength ($W$), quoted in the legend of each subfigure. These results show that all the values of $\langle \sigma_{xy} \rangle$ and $\langle G_{xx} \rangle$, shown in Fig. 5(a) and Fig. 5(b) of the main manuscript, respectively, are independent of $n$. In addition, the error bars for the reported values of $\langle \sigma_{xy} \rangle$ and $\langle G_{xx} \rangle$, corresponding to their standard deviations, are independent of $n$ as well. All the other parameter values are already quoted in the main manuscript.

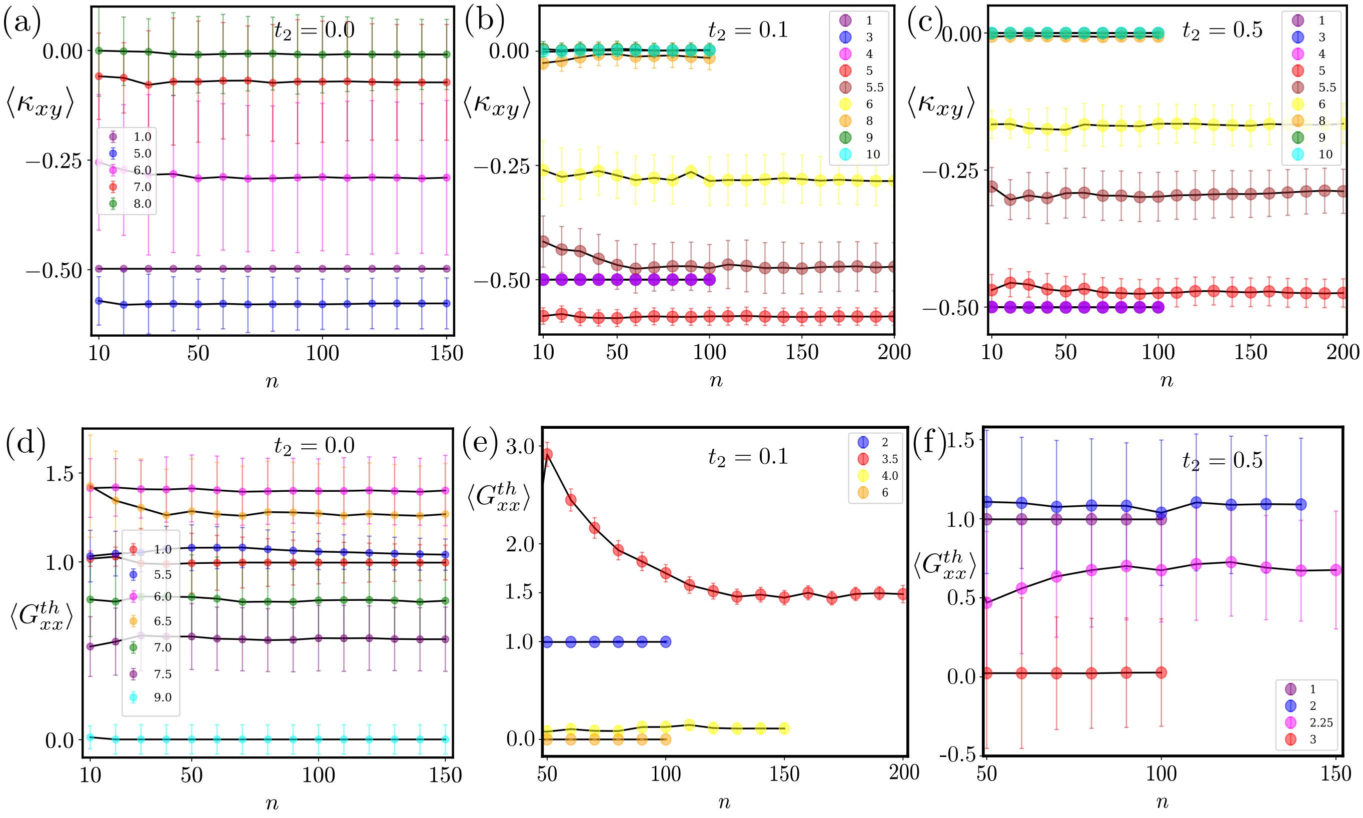


Figure S2. The variation of the disorder-averaged thermal Hall conductivity $\langle\kappa_{xy}\rangle$ in NH $p+ip$ paired state with the number of independent disorder realizations ($n$) for (a) $t_2 = 0.0$, (b) $t_2 = 0.1$, and (c) $t_2 = 0.5$ for a few specific values of the disorder strength ($W$), quoted in the legend of each subfigure. The variation of the disorder-averaged thermal longitudinal conductivity $\langle G^{th}_{xx}\rangle$ in NH $p \pm ip$ paired state with $n$ for (d) $t_2 = 0.0$, (e) $t_2 = 0.1$, and (f) $t_2 = 0.5$ for a few specific values of the disorder strength ($W$), quoted in the legend of each subfigure. These results show that all the values of $\langle\kappa_{xy}\rangle$ and $\langle G^{th}_{xx}\rangle$, shown in Fig. 5(c) and Fig. 5(d) of the main manuscript, respectively, are independent of $n$. In addition, the error bars for the reported values of $\langle\kappa_{xy}\rangle$ and $\langle G^{th}_{xx}\rangle$, representing their standard deviations, are independent of $n$ as well. All the other parameter values are already quoted in the main manuscript.

Electrical/thermal/spin current flows between the leads in the horizonal/longitudinal direction (Lead 1 and Lead 4). It generates a voltage/temperature/magnetization drop in the transverse leads (Lead 2, Lead 3, Lead 5, Lead 6), from which we compute the electrical/thermal/spin transport quantities, described below. See Fig. 1 of the main manuscript for the six-terminal arrangement.

With this set up, we can then obtain the scattering matrix ($S$) by solving the linear equation $\Psi_{\rm out} = S\Psi_{\rm in}$, where

$$S = \begin{pmatrix} r & t' \\ t & r' \end{pmatrix}, \tag{S1}$$

$r$ and $t$ are the reflection and transmission blocks of the scattering matrix, respectively, with $|r|^2 + |t|^2 = 1$, preserving the unitarity of $S$. In our calculations, we take the same lead Hamiltonian as that of the scattering region. Here, $\Psi_{\rm in}$ ($\Psi_{\rm out}$) is the incoming (outgoing) wave function, entering (leaving) the scattering region.

As a longitudinal current flows across the system in presence of an applied electric field $\boldsymbol{E}$, the current-electric field relation reads $j_a = \sum_b \sigma_{ab} E_b$, where $\sigma_{ab}$ is called the conductivity tensor. In our setup, the current is only traversing along the $x$ direction, and thus the Hall conductivity

$$\sigma_{xy} = \frac{j_x E_y}{E_x^2 + E_y^2}, \tag{S2}$$

where $E_x = (V_2 - V_3)/L_{23}$ and $E_y = (V_2 + V_3 - V_5 - V_6)/(2D)$, $L_{23}$ is the distance between Lead 2 and Lead 3, which we set to be $L/5$, and $V_{i=1,\cdots,6}$ are the voltages developed in all the leads (numbered accordingly). The electrical

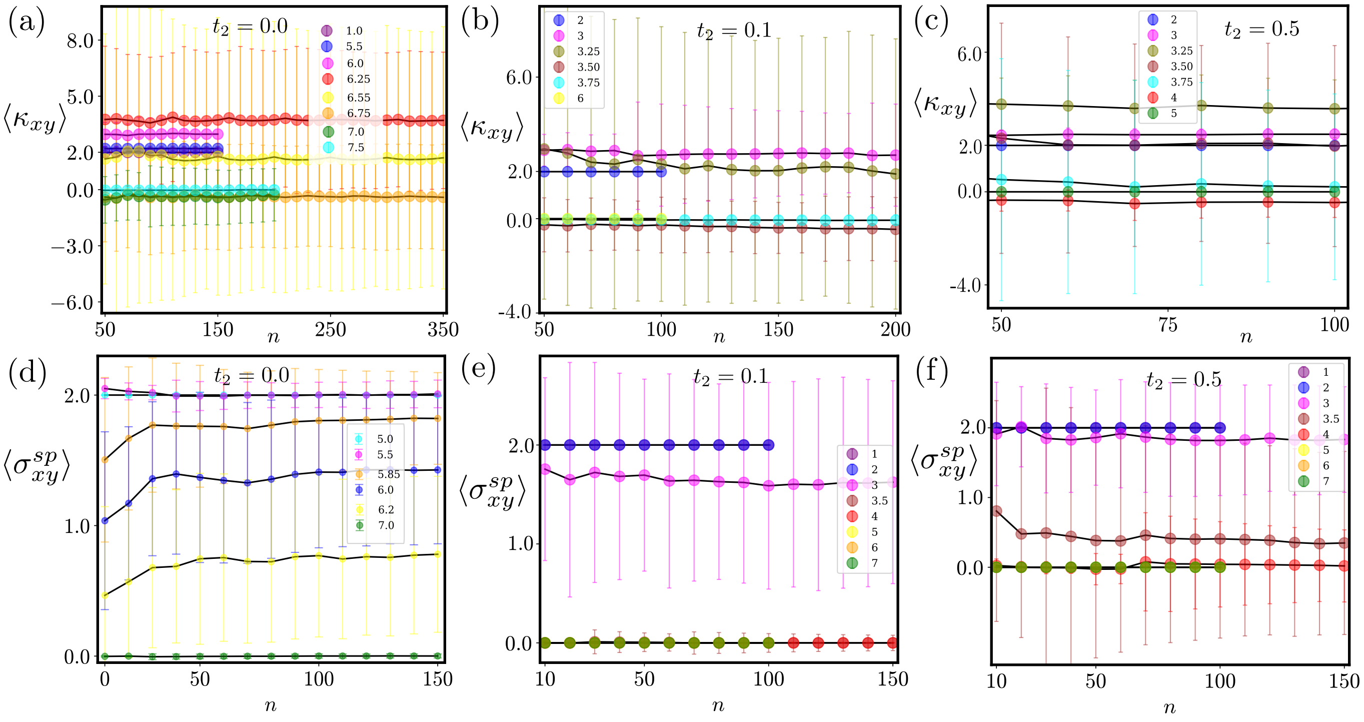


Figure S3. The variation of the disorder-averaged thermal Hall conductivity $\langle \kappa_{xy} \rangle$ in NH $d+id$ superconductor with the number of independent disorder realizations ($n$) for (a) $t_2 = 0.0$, (b) $t_2 = 0.1$, and (c) $t_2 = 0.5$ for a few specific values of the disorder strength ($W$), quoted in the legend of each subfigure. The variation of the disorder-averaged spin Hall conductivity $\langle \sigma^{sp}_{xy} \rangle$ in NH $d+id$ paired state with $n$ for (d) $t_2 = 0.0$, (e) $t_2 = 0.1$, and (f) $t_2 = 0.5$ for a few specific values of the disorder strength ($W$), quoted in the legend of each subfigure. These results show that all the values of $\langle \kappa_{xy} \rangle$ and $\langle \sigma^{sp}_{xy} \rangle$, shown in Fig. 5(e) and Fig. 5(f) of the main manuscript, respectively, are independent of $n$. In addition, the error bars for the reported values of $\langle \kappa_{xy} \rangle$ and $\langle \sigma^{sp}_{xy} \rangle$, corresponding to their standard deviations, are independent of $n$ as well. All the other parameter values are already quoted in the main manuscript.

longitudinal conductivity $G_{xx}$, on the other hand, is obtained from the voltage drop between Lead 2 and Lead 3 or Lead 5 and Lead 6. For the computation of $\kappa_{xy}$ and $G^{th}_{xx}$, a thermal current ($I_{th}$) flows between the horizontal leads. Then $\kappa_{xy}$ is obtained from the temperature drop of the transverse leads and $G^{th}_{xx}$ is obtained from the temperature drop between Lead 2 and Lead 3 or Lead 5 and Lead 6, which are obtained from the linear relation between the thermal current ($\mathbf{I}_{th}$) and temperature ($\mathbf{T}$). In the same setup, for the computation of $\sigma^{sp}_{xy}$, a spin current flows between Lead 1 and Lead 4, which results in a magnetization drop in the vertical leads. In this case, a linear relation between the spin current ($\mathbf{I}_{sp}$) and magnetization ($\mathbf{M}$) is used to extract $\sigma^{sp}_{xy}$. See Figs. 2-5 of the main manuscript for the results in clean system.

## S2. TRANSPORT QUANTITIES IN DISORDERED SYSTEMS

In the main manuscript, we display the disorder-averaged values for the electrical Hall conductivity $\langle \sigma_{xy} \rangle$ for NH quantum anomalous Hall insulator (QAHI), the electrical longitudinal conductivity $\langle G_{xx} \rangle$ for NH quantum spin insulator (QSHI), the thermal Hall conductivity $\langle \kappa_{xy} \rangle$ for NH $p+ip$ paired state, the thermal longitudinal conductivity $\langle G^{th}_{xx} \rangle$ for NH $p \pm ip$ paired state, $\langle \kappa_{xy} \rangle$ for NH $d+id$ paired state, and the spin Hall conductivity $\langle \sigma^{sp}_{xy} \rangle$ for NH $d+id$ paired state, in subfigures (a), (b), (c), (d), (e), and (f) of Fig. 5, respectively. Here we discuss some additional details of those computations that are summarized in Figs. S1, S2 and S3 for a few specific disorder strength $W$.

Firstly, we note that all the quoted values of all the disorder-averaged transport quantities are insensitive to the number of independent disorder realizations $n$, over which such an averaging is performed. Next, we note that the error bar shown for each data point, representing its standard deviation, is also independent of $n$. Finally, we note that the magnitude of the standard deviation is small or negligible when the disorder-averaged transport quantities

are (half-)quantized and zero, realized in the weak and strong disorder regimes, respectively. This is natural to expect as then all the independent disorder realizations yield (half-)quantized and zero values of the associated transport quantities, respectively. By contrast, in the intermediate disorder regime, the standard deviation is typically large, when these quantities acquire non-universal values. This generic observation can be explained by considering one particular example of $\langle \sigma_{xy} \rangle$ in NH QAHI.

Firstly, notice that in units of $e^2/h$ for any given disorder realization $\sigma_{xy} = 1$ or $\sigma_{xy} = 0$. When, for example, $\langle \sigma_{xy} \rangle \approx 0.5$ (in units of $e^2/h$), which can be found in the intermediate disorder regime, for half of the disorder configurations we find $\sigma_{xy} = 1$, while the rests give $\sigma_{xy} = 0$, thereby producing a large standard deviation. However, we ensure that the standard deviations for all reported values of $\langle \sigma_{xy} \rangle$ saturate with respect to the number of disorder configurations ($n$), just like their mean values. The same reasoning and conclusions follow for all the other disorder-averaged transport quantities.
